# Supplementary material for: Higher Martian atmospheric temperatures at all altitudes increase the D/H fractionation factor and water loss
Source: arXiv:2007.12589 ancillary file (2020-10-28)
Supplement: Supplementary file 1 [file Cangi_2020_FF_si_journal_edits.pdf]

# Supporting Information for "Higher Martian atmospheric temperatures at all altitudes increase the D/H fractionation factor and water loss"

E. M. Cangi[1,2], M. S. Chaffin[1], J. Deighan[1]

[1]Laboratory for Atmospheric and Space Physics
[2]University of Colorado Boulder

**Contents of this file**

1. Text S1: Photodissociation cross sections
2. Text S2: Vertical transport
3. Text S3: Boundary conditions
4. Table S1: H chemistry reaction list
5. Table S2: D chemistry reaction list
6. Table S3: Boundary conditions
7. Table S4: Temperature profile parameters
8. Table S5: Fractionation factor results
9. Figure S1: HDO Photodissociation cross section
10. Figure S2: OH Photodissociation cross section
11. Figure S3: Reproductions of past studies
12. Figure S4: Contributions of atomic and molecular H, D to loss of H, D
13. Figure S5: Thermal and non-thermal contributions to escape fluxes of H and D for tropopause and exobase temperature variations
14. Figure S6: Changes in transport flux and chemical production/loss of D and H by altitude and tropopause temperature
15. Figure S7: Changes in transport flux and chemical production/loss of D and H by altitude and exobase temperature

**Introduction**

This Supporting Information file provides additional information on parameters of the model in Text S1-S3, Figures S1-S3, and Tables S1-S4. A numerical table of the results in Figure 4 appears in Table S5. Figures S4-S7 provide additional context supporting the discussion points and conclusions.

**Text S1. Photodissociation cross sections**

Photodissociation is the process by which molecules are dissociated due to absorption of incoming solar photons. A key parameter that governs absorption of these photons is the photochemical cross section of the absorber; unfortunately, measurements on photochemical cross sections for D-bearing species are rare and incomplete in the literature. In this work, we have included cross sections for semi-heavy water (HDO) (Cheng et al., 1999, 2004), shown in Figure S1, and deuterated hydroxyl (OD) (Nee & Lee, 1984), shown in Figure S2. The OD cross sections are only available for a small wavelength range compared to OH, so we fill in gaps for OD using the OH data. For the HDO cross sections, we use the measurements valid for 298-300 K, which are the most complete available Cheng et al. (1999, 2004). A less complete

Corresponding author: E. M. Cangi, Laboratory for Atmospheric and Space Physics, Boulder, CO 80301, USA. (eryn.cangi@lasp.colorado.edu)

data set exists for 250 K. Ideally, HDO cross section data in the range of 150-250 K would be used, but these measurements do not exist in the literature. For our purposes, the 300 K cross sections are sufficient, at least until some point in the future when more measurements will hopefully be made.

**Text S2. Vertical transport**

In terms of modeling the martian atmosphere, the most important distinction between eddy and molecular diffusion are the regimes in which they dominate. Turbulent mixing dominates in the lower atmosphere, and is approximated using eddy diffusion. In this regime, molecular species are intermixed and do not stratify due to their masses. We use the following piece-wise equation for eddy diffusion:

$$K = \begin{cases} 10^6 & z < 60 \text{ km} \\ 2 \times 10^{13} n^{-1/2} & z > 60 \text{ km} \end{cases}$$

Where $n$ is the total number of particles in the atmosphere layer. A similar equation is used by V. Krasnopolsky (2000) and Chaffin, Deighan, Schneider, and Stewart (2017).

Above the homopause (about 120 km), molecular diffusion dominates, meaning that molecular species diffusively separate and follow their own scale heights. Molecular diffusion is described by the following equation from Banks and Kockarts (1973):

$$D = \frac{AT^s}{n} \tag{1}$$

The values of $A$ and $s$ for H and $H_2$ through $CO_2$ have been experimentally determined (Hunten, 1973): $A_H = 8.4 \times 10^{17}$, $s_H = 0.597$, $A_{H_2} = 2.23 \times 10^{17}$, $s_{H_2} = 0.75$. For D and HD, we used the theoretical framework for determining $A$ and $s$ given by Banks and Kockarts (1973). This framework applied to H and $H_2$ results in values of $A$ that disagree with experiment, so we first calculate $A$ and $s$ for D and HD, then use the ratio of the experimental and theoretical values for H and $H_2$ to scale them, giving the results: $A_D = 5.98 \times 10^{17}$, $A_{HD} = 1.84 \times 10^{17}$. For $s_D$ and $s_{HD}$, we use the same values as the H-bearing species. For other species, experimental data of $A$ and $s$ are not readily available. We set $A$ and $s$ for other species to 1 and 0.75 respectively, as they should diffuse less easily compared to H, D, $H_2$ and HD.

**Text S3. Boundary conditions**

In general, we use the same boundary conditions used by Chaffin et al. (2017), given in Table S3. Densities of Ar and $N_2$ are fixed to be 2% and 1.9% of the $CO_2$ density respectively. All surface-ward fluxes are fixed to be 0 as we do not account for surface deposition in our model; surface deposition is likely an important process, however, and has been explored in other studies (Zahnle et al., 2008). Because we are only modeling thermal escape, we assume that no species more massive than HD is able to escape to space, and therefore flux to space for more massive species is 0 (except for the flux of O, which is fixed as shown in the table).

**References**


Banks, P. M., & Kockarts, G. (1973). *Aeronomy.* Academic Press, Inc.

Barfield, W., Koontz, G., & Huebner, W. (1972). Fits to new calculations of photoionization cross sections for low-z elements. *Journal of Quantitative Spectroscopy and Radiative Transfer*, *12*. doi: 10.1016/0022-4073(72)90043-X

Cazaux, S., Cobut, V., Marseille, M., Spaans, M., & Caselli, P. (2010). Water formation on bare grains: When the chemistry on dust impacts interstellar gas. *Astronomy & Astrophysics*, *522*. doi: 10.1051/0004-6361/201014026

Chaffin, M. S., Deighan, J., Schneider, N. M., & Stewart, A. I. F. (2017). Elevated atmospheric escape of atomic hydrogen from Mars induced by high-altitude water. *Nature Geoscience*, *10*. doi: 10.1038/ngeo2887

Cheng, B. M., Chew, E. P., Liu, C. P., et al. (1999). Photo-induced fractionation of water isotopomers in the Martian atmosphere. *Geophysical Research Letters*, *26*. doi: 10.1029/1999GL008367

Cheng, B. M., Chung, C. Y., Bahou, M., Lee, Y. P., Lee, L. C., Van Harrevelt, R., & Van Hemert, M. C. (2004). Quantitative spectroscopic and theoretical study of the optical absorption spectra of H 2O, HOD, and D 2O in the 125-145 nm region. *Journal of Chemical Physics*, *120*. doi: 10.1063/1.1630304

Deighan, J. (2012). *The effect of an ozone layer on ancient mars* (Doctoral dissertation, University of Virginia). Retrieved from `http://libra.virginia.edu/catalog/libra-oa:2577`

Hunten, D. M. (1973). The Escape of Light Gases from Planetary Atmospheres. *Journal of the Atmospheric Sciences*, *30*. doi: 10.1016/0032-0633(82)90110-6

Krasnopolsky, V. (2000). On the Deuterium Abundance on Mars and Some Related Problems. *Icarus*, *148*. doi: 10.1006/icar.2000.6534

Krasnopolsky, V. A. (2002). Mars' upper atmosphere and ionosphere at low, medium, and high solar activities: Implications for evolution of water. *Journal of Geophysical Research: Planets*, *107*. doi: 10.1029/2001JE001809

Krasnopolsky, V. A. (2010). Solar activity variations of thermospheric temperatures on Mars and a problem of CO in the lower atmosphere. *Icarus*, *207*. doi: 10.1016/j.icarus.2009.12.036

Manion, J. A., Huie, R. E., Levin, R. D., Burgess Jr., D. R., Orkin, V. L., Tsang, W., ... Frizzell, D. H. (2015). *NIST Chemical Kinetics Database.* Retrieved 2015-09, from `http://kinetics.nist.gov/`

Nee, J. B., & Lee, L. C. (1984). Photoabsorption cross section of OD at 115-180 nm. *The Journal of Chemical Physics*, *81*. doi: 10.1063/1.448183

Sander, S. P., Friedl, R. R., Golden, D. M., Kurylo, M. J., Moortgat, G. K., Wine, P. H., ... Orkin, V. L. (2011). Chemical Kinetics and Photochemical Data for Use in Atmospheric Studies Evaluation Number 15. *Cross Sections*. doi: 10.1002/kin.550171010

Wakelam, V., & Gratier, P. (2019). *Kinetic Database for Astrochemistry.* Retrieved from `http://kida.obs.u-bordeaux1.fr/contact.html`

Yung, Y. L., Wen, J.-S., Moses, J. I., Landry, B. M., Allen, M., & Hsu, K.-J. (1989). Hydrogen and deuterium loss from the terrestrial atmosphere: A quantitative assessment of nonthermal escape fluxes. *Journal of Geophysical Research*, *94*.

Yung, Y. L., Wen, J. S., Pinto, J. P., Allen, M., Pierce, K. K., & Paulson, S. (1988). HDO in the Martian atmosphere: Implications for the abundance of crustal water. *Icarus*, *76*. doi: 10.1016/0019-1035(88)90147-9

Zahnle, K., Haberle, R. M., Catling, D. C., & Kasting, J. F. (2008). Photochemical instability of the ancient Martian atmosphere. *Journal of Geophysical Research E: Planets*, *113*. doi: 10.1029/2008JE003160

Table S1: H-bearing chemical reactions used in the model. For the photodissociation reactions (unimolecular reactions), the entry in the rate coefficient column is the total model-calculated rate at the top of the equilibrated atmosphere for the standard temperature profile, as reference. For bimolecular reactions, the rate coefficient is in units of $cm^3$ $molecule^{-1}$ $s^{-1}$. For termolecular reactions, the unit is $cm^6$ $molecule^{-1}$ $s^{-1}$.

| Number | Reaction | Rate coefficient | Ref |
|---|---|---|---|
| R1a | $CO_2 \rightarrow CO + O$ | $6.1 \times 10^{-8}$ | |
| R1b | $\rightarrow CO + O(^1D)$ | $2.4 \times 10^{-7}$ | |
| R2a | $O_2 \rightarrow O + O$ | $2.3 \times 10^{-8}$ | |
| R2b | $\rightarrow O + O(^1D)$ | $4.7 \times 10^{-7}$ | |
| R3a | $O_3 \rightarrow O_2 + O$ | $2.5 \times 10^{-4}$ | |
| R3b | $\rightarrow O_2 + O(^1D)$ | $1.5 \times 10^{-3}$ | |
| R4 | $H_2 \rightarrow H + H$ | $1.2 \times 10^{-8}$ | |
| R5a | $OH \rightarrow O + H$ | $1.4 \times 10^{-6}$ | |
| R5b | $\rightarrow O(^1D) + H$ | $4.2 \times 10^{-8}$ | |
| R6 | $HO_2 \rightarrow OH + O$ | $1.0 \times 10^{-4}$ | |
| R7a | $H_2O \rightarrow H + OH$ | $1.9 \times 10^{-6}$ | |
| R7b | $\rightarrow H_2 + O(^1D)$ | $1.2 \times 10^{-7}$ | |
| R8a | $H_2O_2 \rightarrow OH + OH$ | $1.8 \times 10^{-5}$ | |
| R8b | $\rightarrow HO_2 + H$ | $9.4 \times 10^{-7}$ | |
| R9 | $O + O + M \rightarrow O_2 + M$ | $5.4 \times 10^{-33}(300/T)^{3.25}$ | *d* |
| R10 | $O + O_2 + N_2 \rightarrow O_3 + N_2$ | $5 \times 10^{-35}e^{724/T}$ | *a* |
| R11 | $O + O_2 + CO_2 \rightarrow O_3 + CO_2$ | $1.5 \times 10^{-33}(300/T)^{2.4}$ | *a* |
| R12 | $O + O_3 \rightarrow O_2 + O_2$ | $8.0 \times 10^{-12}e^{-2060/T}$ | *a* |
| R13 | $O + CO + M \rightarrow CO_2 + M$ | $2.2 \times 10^{-33}e^{-1780/T}$ | *d* |
| R14 | $O(^1D) + O_2 \rightarrow O + O_2$ | $3.2 \times 10^{-11}e^{70/T}$ | *a* |
| R15 | $O(^1D) + O_3 \rightarrow O_2 + O_2$ | $1.2 \times 10^{-10}$ | *a* |
| R16 | $\rightarrow O + O + O_2$ | $1.2 \times 10^{-10}$ | *a* |
| R17 | $O(^1D) + CO_2 \rightarrow O + CO_2$ | $7.5 \times 10^{-11}e^{115/T}$ | *a* |
| R18 | $O(^1D) + H_2 \rightarrow H + OH$ | $1.2 \times 10^{-10}$ | *a* |
| R19 | $O(^1D) + H_2O \rightarrow OH + OH$ | $1.63 \times 10^{-10}e^{60/T}$ | *a* |
| R20 | $H_2 + O \rightarrow OH + H$ | $6.34 \times 10^{-12}e^{-4000/T}$ | *b* |
| R21 | $OH + H_2 \rightarrow H_2O + H$ | $2.8 \times 10^{-12}e^{-1800/T}$ | *a* |
| R22 | $H + H + M \rightarrow H_2 + M$ | $1.6 \times 10^{-32}\left(\frac{298}{T}\right)^{2.27}$ | *d* |
| R23 | $H + OH + CO_2 \rightarrow H_2O + CO_2$ | $1.292 \times 10^{-30}\left(\frac{300}{T}\right)^{2}$ | *c* |
| R24a | $H + HO_2 \rightarrow OH + OH$ | $7.2 \times 10^{-11}$ | *a* |
| R24b | $\rightarrow H_2 + O_2$ | $3.45 \times 10^{-12}$ | *a* |
| R24c | $\rightarrow H_2O + O(^1D)$ | $1.6 \times 10^{-12}$ | *a* |
| R25a | $H + H_2O_2 \rightarrow HO_2 + H_2$ | $2.81 \times 10^{-12}e^{-1890/T}$ | *c* |
| R25b | $\rightarrow H_2O + OH$ | $1.7 \times 10^{-11}e^{-1800/T}$ | *c* |

Continued on next page

Table S1 – continued from previous page

| Number | Reaction | Rate coefficient | Ref |
|---|---|---|---|
| R26 | $H + O_2 \rightarrow HO_2$ | $k_0 = 8.8 \times 10^{-32} \left(\frac{T}{300}\right)^{-1.3}$ | *ad* |
| | | $k_\infty = 7.5 \times 10^{-11} \left(\frac{T}{300}\right)^{0.2}$ | *ad* |
| R27 | $H + O_3 \rightarrow OH + O_2$ | $1.4 \times 10^{-10} e^{-470/T}$ | *c* |
| R28 | $O + OH \rightarrow O_2 + H$ | $1.8 \times 10^{-11} e^{180/T}$ | *a* |
| R29 | $O + HO_2 \rightarrow OH + O_2$ | $3.0 \times 10^{-11} e^{200/T}$ | *a* |
| R30 | $O + H_2O_2 \rightarrow OH + HO_2$ | $1.4 \times 10^{-12} e^{-2000/T}$ | *a* |
| R31a | $OH + OH \rightarrow H_2O + O$ | $4.2 \times 10^{-12} e^{-240/T}$ | *c* |
| R31b | $\rightarrow H_2O_2$ | $k_0 = 8.97 \times 10^{-31} \left(\frac{T}{300}\right)^{-1.0}$ | *ad* |
| | | $k_\infty = 2.6 \times 10^{-11}$ | *ad* |
| R32 | $OH + O_3 \rightarrow HO_2 + O_2$ | $1.7 \times 10^{-12} e^{-940/T}$ | *a* |
| R33 | $OH + HO_2 \rightarrow H_2O + O_2$ | $4.8 \times 10^{-11} e^{250/T}$ | *a* |
| R34 | $OH + H_2O_2 \rightarrow H_2O + HO_2$ | $2.9 \times 10^{-12} e^{-160/T}$ | *c* |
| R35 | $HO_2 + O_3 \rightarrow OH + O_2 + O_2$ | $1.0 \times 10^{-14} e^{-490/T}$ | *a* |
| R36 | $HO_2 + HO_2 \rightarrow H_2O_2 + O_2$ | $3.0 \times 10^{-13} e^{460/T}$ | *a* |
| R37 | $HO_2 + HO_2 + M \rightarrow H_2O_2 + O_2 + M$ | $4.2 \times 10^{-33} e^{920/T}$ | *a* |
| R38 | $CO + OH \rightarrow CO_2 + H$ | $k_0 = 1.5 \times 10^{-13} \left(\frac{T}{300}\right)^{0.6}$ | *a* |
| | | $k_\infty = 2.1 \times 10^{9} \left(\frac{T}{300}\right)^{6.1}$ | *a* |
| R39 | $OH + CO \rightarrow CO_2H$ | $k_0 = 5.9 \times 10^{-33} \left(\frac{T}{300}\right)^{-1.4}$ | *a* |
| | | $k_\infty = 1.1 \times 10^{-12} \left(\frac{T}{300}\right)^{1.3}$ | *a* |
| R40 | $CO_2H + O_2 \rightarrow HO_2 + CO_2$ | $2.09 \times 10^{-12}$ | *c* |
| R41 | $CO_2^+ + H_2 \rightarrow CO_2 + H + H$ | $8.7 \times 10^{-10}$ | *e* |

[a]Sander et al. (2011). [b]KIDA database (Wakelam & Gratier, 2019).
[c]NIST database (Manion et al., 2015). [d] Deighan (2012). [e]V. A. Krasnopolsky (2010).

Table S2: The same as Table S1, but for D-bearing chemistry. Where we cite *a*, we multiply the H-bearing reaction in Table S1 by the multiplier specified in *a*. If the reference specifies a different rate entirely, we use it. Reaction numbers have been chosen so that the reaction of the same number in Table S1 is the H-bearing analogue reaction.

| Number | Reaction | Rate | Ref |
|---|---|---|---|
| DR4 | $HD \rightarrow H + D$ | $1.2 \times 10^{-8}$ | |
| DR5a | $OD \rightarrow O + D$ | $2.3 \times 10^{-6}$ | |
| DR5b | $\rightarrow O(^1D) + D$ | $4.2 \times 10^{-8}$ | |
| DR6 | $DO_2 \rightarrow OD + O$ | $1.0 \times 10^{-4}$ | |
| DR7a | $HDO \rightarrow H + OD$ | $6.3 \times 10^{-7}$ | |
| DR7b | $\rightarrow D + OH$ | $6.3 \times 10^{-7}$ | |
| DR7c | $\rightarrow HD + O(^1D)$ | $4.3 \times 10^{-8}$ | |
| DR8a | $HDO_2 \rightarrow OH + OD$ | $1.8 \times 10^{-5}$ | |
| DR8b | $\rightarrow DO_2 + H$ | $4.7 \times 10^{-7}$ | |
| DR8c | $\rightarrow HO_2 + D$ | $4.7 \times 10^{-7}$ | |
| DR18a | $O(^1D) + HD \rightarrow H + OD$ | $4.92 \times 10^{-11}$ | *a* |
| DR18b | $\rightarrow D + OH$ | $4.92 \times 10^{-11}$ | *a* |
| DR19 | $O(^1D) + HDO \rightarrow OD + OH$ | $1.63 \times 10^{-10} e^{60/T}$ | *a* |
| DR20a | $HD + O \rightarrow OH + D$ | $4.40 \times 10^{-12} e^{-4390/T}$ | *b* |
| DR20b | $\rightarrow OD + H$ | $1.68 \times 10^{-12} e^{-4400/T}$ | *b* |
| DR21a | $OH + HD \rightarrow HDO + H$ | $(3/20) 2.8 \times 10^{-12} e^{-1800/T}$ | *a* |
| DR21b | $\rightarrow H_2O + D$ | $(3/20) 2.8 \times 10^{-12} e^{-1800/T}$ | *a* |
| DR21c | $OD + H_2 \rightarrow HDO + H$ | $2.8 \times 10^{-12} e^{-1800/T}$ | *a* |
| DR22 | $H + D + M \rightarrow HD + M$ | $1.6 \times 10^{-32} \left(\frac{298}{T}\right)^{2.27}$ | *a* |
| DR23a | $H + OD + CO_2 \rightarrow HDO + CO_2$ | $1.292 \times 10^{-30} \left(\frac{300}{T}\right)^{2}$ | * |
| DR23b | $D + OH + CO_2 \rightarrow HDO + CO_2$ | $1.292 \times 10^{-30} \left(\frac{300}{T}\right)^{2}$ | * |
| DR24a | $H + DO_2 \rightarrow OH + OD$ | $7.2 \times 10^{-11}$ | *a* |
| DR24b | $\rightarrow HD + O_2$ | $3.45 \times 10^{-12}$ | *a* |
| DR24c | $\rightarrow HDO + O(^1D)$ | $1.6 \times 10^{-12}$ | *a* |
| DR24d | $\rightarrow HO_2 + D$ | $1 \times 10^{-10} / (0.54 e^{890/T})$ | *a* |
| DR24e | $D + HO_2 \rightarrow OH + OD$ | $5.112 \times 10^{-11}$ | *a* |
| DR24f | $\rightarrow HD + O_2$ | $2.4495 \times 10^{-12}$ | *a* |
| DR24g | $\rightarrow HDO + O(^1D)$ | $1.136 \times 10^{-12}$ | *a* |
| DR24h | $\rightarrow DO_2 + H$ | $1.0 \times 10^{-10}$ | *a* |
| DR25a | $H + HDO_2 \rightarrow HDO + OH$ | $5.8 \times 10^{-10} e^{-2110/T}$ | *c* |
| DR25b | $\rightarrow H_2O + OD$ | $5.8 \times 10^{-10} e^{-2110/T}$ | *c* |
| DR25c | $D + H_2O_2 \rightarrow HDO + OH$ | $5.8 \times 10^{-10} e^{-2110/T}$ | *c* |
| DR25d | $\rightarrow H_2O + OD$ | $5.8 \times 10^{-10} e^{-2110/T}$ | *c* |
| DR25e | $D + HDO_2 \rightarrow OD + HDO$ | $5.8 \times 10^{-10} e^{-2110/T}$ | *c* |
| DR26 | $D + O_2 \rightarrow DO_2$ | $k_0 = 8.8 \times 10^{-32} \left(\frac{T}{300}\right)^{-1.3}$ | *a* |

Continued on next page

Table S2 – continued from previous page

| Number | Reaction | Rate | Ref |
|---|---|---|---|
| | | $k_\infty = 7.5 \times 10^{-11} \left(\frac{T}{300}\right)^{0.2}$ | a |
| DR27 | $D + O_3 \rightarrow OD + O_2$ | $9.94 \times 10^{-11} e^{-470/T}$ | a |
| DR28 | $O + OD \rightarrow O_2 + D$ | $1.8 \times 10^{-11} e^{180/T}$ | a |
| DR29 | $O + DO_2 \rightarrow OD + O_2$ | $3.0 \times 10^{-11} e^{200/T}$ | a |
| DR30a | $O + HDO_2 \rightarrow OD + HO_2$ | $0.7 \times 10^{-12} e^{-2000/T}$ | a |
| DR30b | $\rightarrow OH + DO_2$ | $0.7 \times 10^{-12} e^{-2000/T}$ | a |
| DR31a | $OD + OH \rightarrow HDO + O$ | $4.2 \times 10^{-12} e^{-240/T}$ | a |
| DR31b | $\rightarrow HDO_2$ | $k_0 = 8.97 \times 10^{-31} \left(\frac{T}{300}\right)^{-1.0}$ | a |
| | | $k_\infty = 2.6 \times 10^{-11}$ | a |
| DR32 | $OD + O_3 \rightarrow DO_2 + O_2$ | $1.7 \times 10^{-12} e^{-940/T}$ | a |
| DR33a | $OH + DO_2 \rightarrow HDO + O_2$ | $4.8 \times 10^{-11} e^{250/T}$ | a |
| DR33b | $OD + HO_2 \rightarrow HDO + O_2$ | $4.8 \times 10^{-11} e^{250/T}$ | a |
| DR34a | $OD + H_2O_2 \rightarrow HDO + HO_2$ | $2.9 \times 10^{-12} e^{-160/T}$ | a |
| DR34b | $OH + HDO_2 \rightarrow HDO + HO_2$ | $1.45 \times 10^{-12} e^{-160/T}$ | a |
| DR34c | $\rightarrow H_2O + DO_2$ | $1.45 \times 10^{-12} e^{-160/T}$ | a |
| DR35 | $DO_2 + O_3 \rightarrow OD + O_2 + O_2$ | $1.0 \times 10^{-14} e^{-490/T}$ | a |
| DR36 | $DO_2 + HO_2 \rightarrow HDO_2 + O_2$ | $3.0 \times 10^{-13} e^{460/T}$ | a |
| DR37 | $HO_2 + DO_2 + M \rightarrow HDO_2 + O_2 + M$ | $4.2 \times 10^{-33} e^{920/T}$ | * |
| DR38 | $CO + OD \rightarrow CO_2 + D$ | $k_0 = 1.5 \times 10^{-13} \left(\frac{T}{300}\right)^{0.6}$ | a |
| | | $k_\infty = 2.1 \times 10^{-9} \left(\frac{T}{300}\right)^{6.1}$ | a |
| DR39 | $CO + OD \rightarrow CO_2D$ | $k_0 = 5.9 \times 10^{-33} \left(\frac{T}{300}\right)^{-1.4}$ | * |
| | | $k_\infty = 1.1 \times 10^{-12} \left(\frac{T}{300}\right)^{1.3}$ | * |
| DR40 | $CO_2D + O_2 \rightarrow DO_2 + CO_2$ | $2.09 \times 10^{-12}$ | * |
| DR41 | $CO_2^+ + HD \rightarrow CO_2^+ + H + D$ | $(2/5)\, 8.7 \times 10^{-10}$ | a |
| DR42a | $H + HD \rightarrow H_2 + D$ | $6.31 \times 10^{-11} e^{-4038/T}$ | d |
| DR42b | $D + H_2 \rightarrow HD + H$ | $6.31 \times 10^{-11} e^{-3821/T}$ | b |
| DR43a | $OD + H \rightarrow OH + D$ | $3.3 \times 10^{-9} (T^{-0.63}) / (0.72 e^{717/T})$ | a |
| DR43b | $OH + D \rightarrow OD + H$ | $3.3 \times 10^{-9} T^{-0.63}$ | a |

[a]Yung et al. (1988). [b]NIST database (Manion et al., 2015). [c](Cazaux et al., 2010). [d](Yung et al., 1989). *No source found. Assumed same rate as H-bearing reaction.

**Table S3.** Boundary Conditions

| Species | Surface density ($cm^{-3}$) | Surface flux ($cm^{-2}s^{-1}$) | Flux to space ($cm^{-2}s^{-1}$) | Outgoing velocity[a] (cm/s) |
|---|---|---|---|---|
| $CO_2$ | $2.1 \times 10^{17}$ | - | 0 | - |
| Ar | $2.0 \times 10^{-2}(2.1 \times 10^{17})$ | - | 0 | - |
| $N_2$ | $1.9 \times 10^{-2}(2.1 \times 10^{17})$ | - | 0 | - |
| $H_2O$ | Set by vapor pressure | - | 0 | - |
| HDO | Set by vapor pressure | - | 0 | - |
| O | - | 0 | $1.2 \times 10^8$ | - |
| H | - | 0 | - | 402 |
| D | - | 0 | - | 0.5 |
| $H_2$ | - | 0 | - | 0.5 |
| HD | - | 0 | - | $6 \times 10^{-4}$ |

[a]Outgoing velocity is fixed to the effusion velocity (Hunten, 1973), which depends on the exobase temperature. Values quoted here are for the nominal exobase temperature used in the model, $T_{exo} = 205$K, but each model run uses an effusion velocity appropriate to its exobase temperature.

**Table S4.** Parameters for temperature profiles

| Profile | $T_{surf}$ (K) | $T_{tropo}$ (K) | $T_{exo}$ (K) |
|---|---|---|---|
| Mean | 216 | 130 | 205 |
| Cold surface | 160 | 130 | 205 |
| Warm surface | 270 | 130 | 205 |
| Cold tropopause | 216 | 100 | 205 |
| Warm tropopause | 216 | 160 | 205 |
| Cold exobase | 216 | 130 | 150 |
| Warm exobase | 216 | 130 | 250 |

**Table S5.** Fractionation factor results as a function of atmospheric parameter. Reported values of $f$ are the minimum and maximum calculated within the range of the varied parameter.

| | Thermal | | Non-thermal | | All escape | |
|---|---|---|---|---|---|---|
| Parameter varied | $f_{min}$ | $f_{max}$ | $f_{min}$ | $f_{max}$ | $f_{min}$ | $f_{max}$ |
| Surface temperature | 0.0014 | 0.0020 | 0.34 | 0.50 | 0.04 | 0.06 |
| Tropopause temperature | 0.0009 | 0.0035 | 0.26 | 0.86 | 0.03 | 0.10 |
| Exobase temperature | $3.3 \times 10^{-5}$ | 0.0172 | 0.48 | 0.81 | 0.06 | 0.1 |
| Water vapor | 0.0015 | 0.0020 | 0.39 | 0.50 | 0.05 | 0.06 |

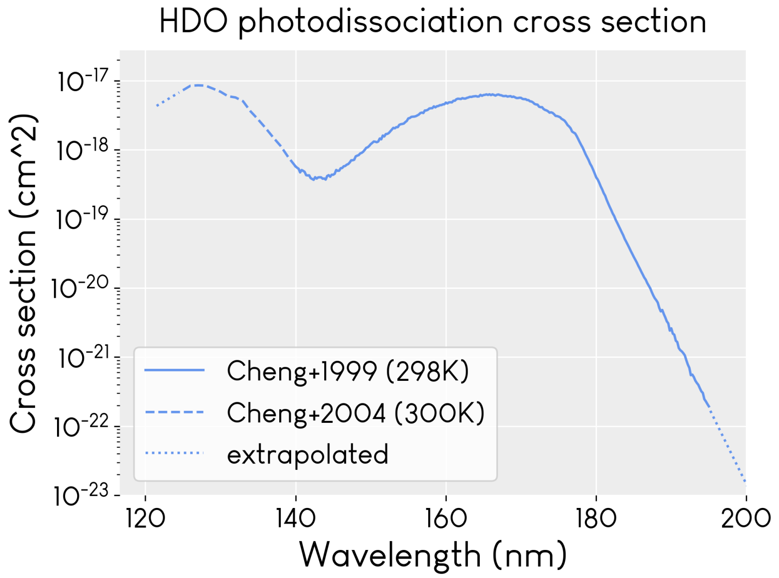


**Figure S1.** HDO cross sections used in this work, collected from Cheng et al. (1999, 2004), the studies with the most complete data available, despite the temperature of measurement (298-300 K) being a bit high for the Martian atmosphere. We extrapolate the data at the edges of the data set in order to have cross sections available for all necessary wavelengths in the model.

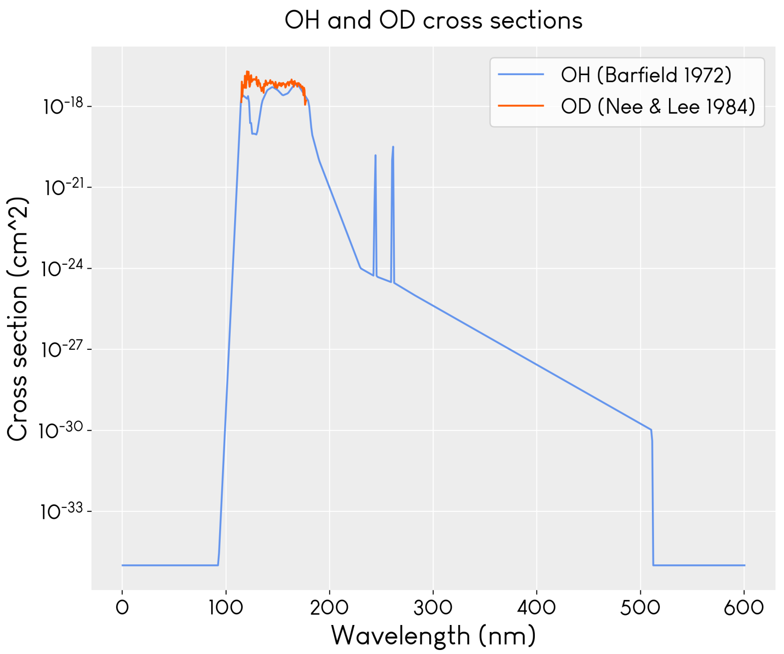


**Figure S2.** OD and OH cross sections used in this work. The OH cross sections are from Barfield et al. (1972), while the few OD cross sections are from Nee and Lee (1984). We use cross section data for OD in the wavelengths available, and the OH cross section everywhere else.

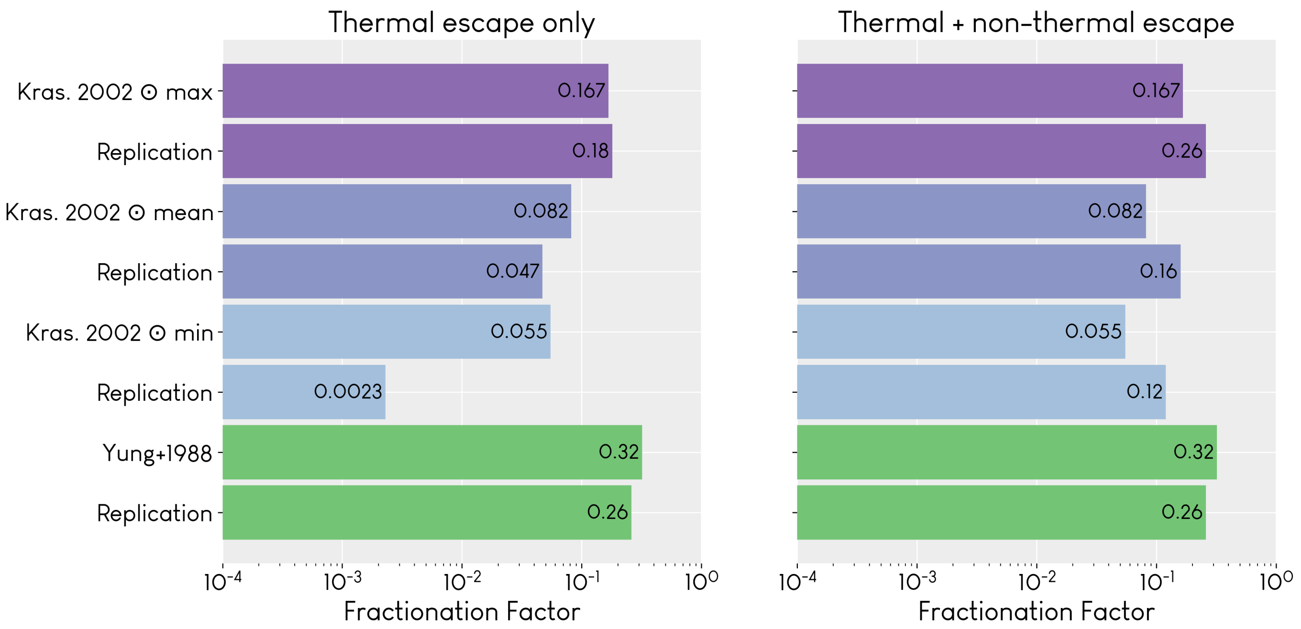


**Figure S3.** Reproductions of past studies that obtained a value of the fractionation factor. a) For thermal escape only. The best agreement is with Yung et al. (1988), which also only considered thermal escape. b) For both thermal and non-thermal escape. The non-thermal escape contribution is the same as in V. A. Krasnopolsky (2002), and is added on to this study's thermal-only reproduction. Inclusion of non-thermal escape improves the agreement with V. A. Krasnopolsky (2002) at solar minimum, when the exobase is cold (below 270 K) and non-thermal escape processes dominate for D, HD, and $H_2$.

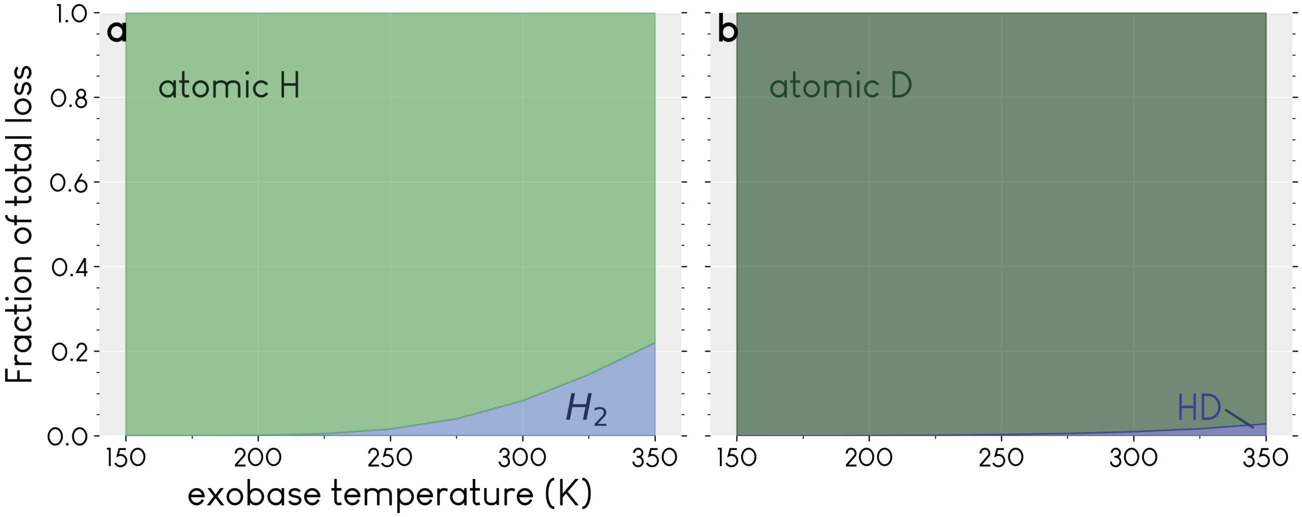


**Figure S4.** Contributions of the atomic and molecular forms to the overall thermal escape of (a) H and (b) D. High temperatures are required to remove the molecular forms, whereas at low temperatures, loss via the atomic forms is near 100%. HD can contribute to H loss, but the fraction is so small ($\sim 10^{-10}$) as to be completely negligible.

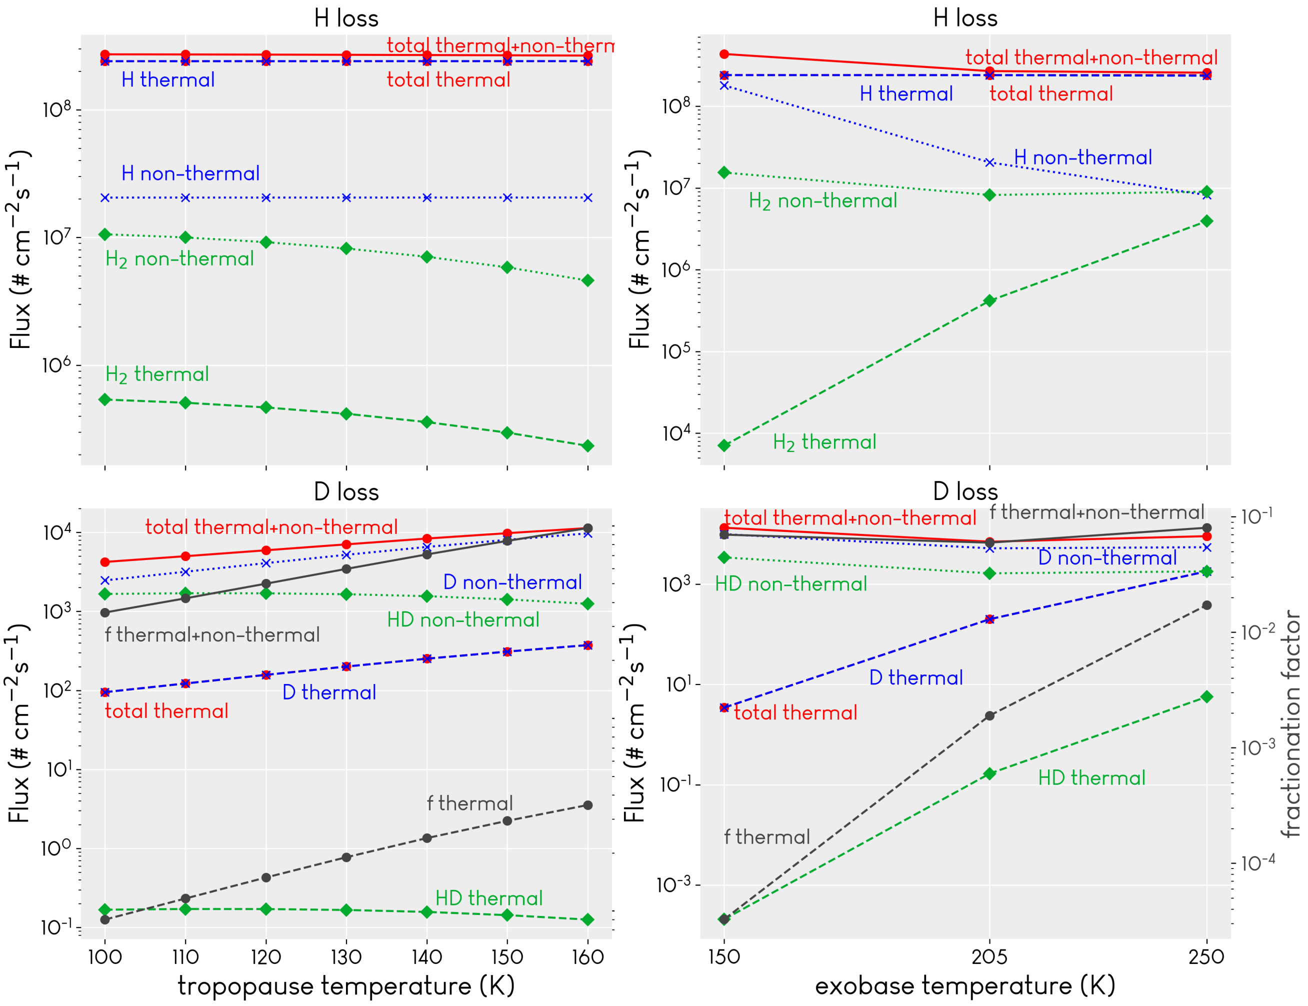


**Figure S5.** Modeled thermal and estimated non-thermal contributions to escape fluxes of H and D (panels a and b) for simulations where either the tropopause (panels a and c) or exobase (panels b and d) temperatures were varied. Each point represents a single simulation. The simulation's calculated fractionation factor $f$ is plotted on the secondary (gray) axis of panels c and d. In panels a and c, each simulation uses standard atmosphere exobase temperature (205 K). In panels b and d, each simulation uses the standard atmosphere tropopause temperature (130 K). Because the exobase temperature varies in panels b and d, and because our estimates for non-thermal escape were based on other simulations by V. A. Krasnopolsky (2002) (which did not extend down below 200 K), it is likely that our estimates for non-thermal escape at low exobase temperatures are artificially high.

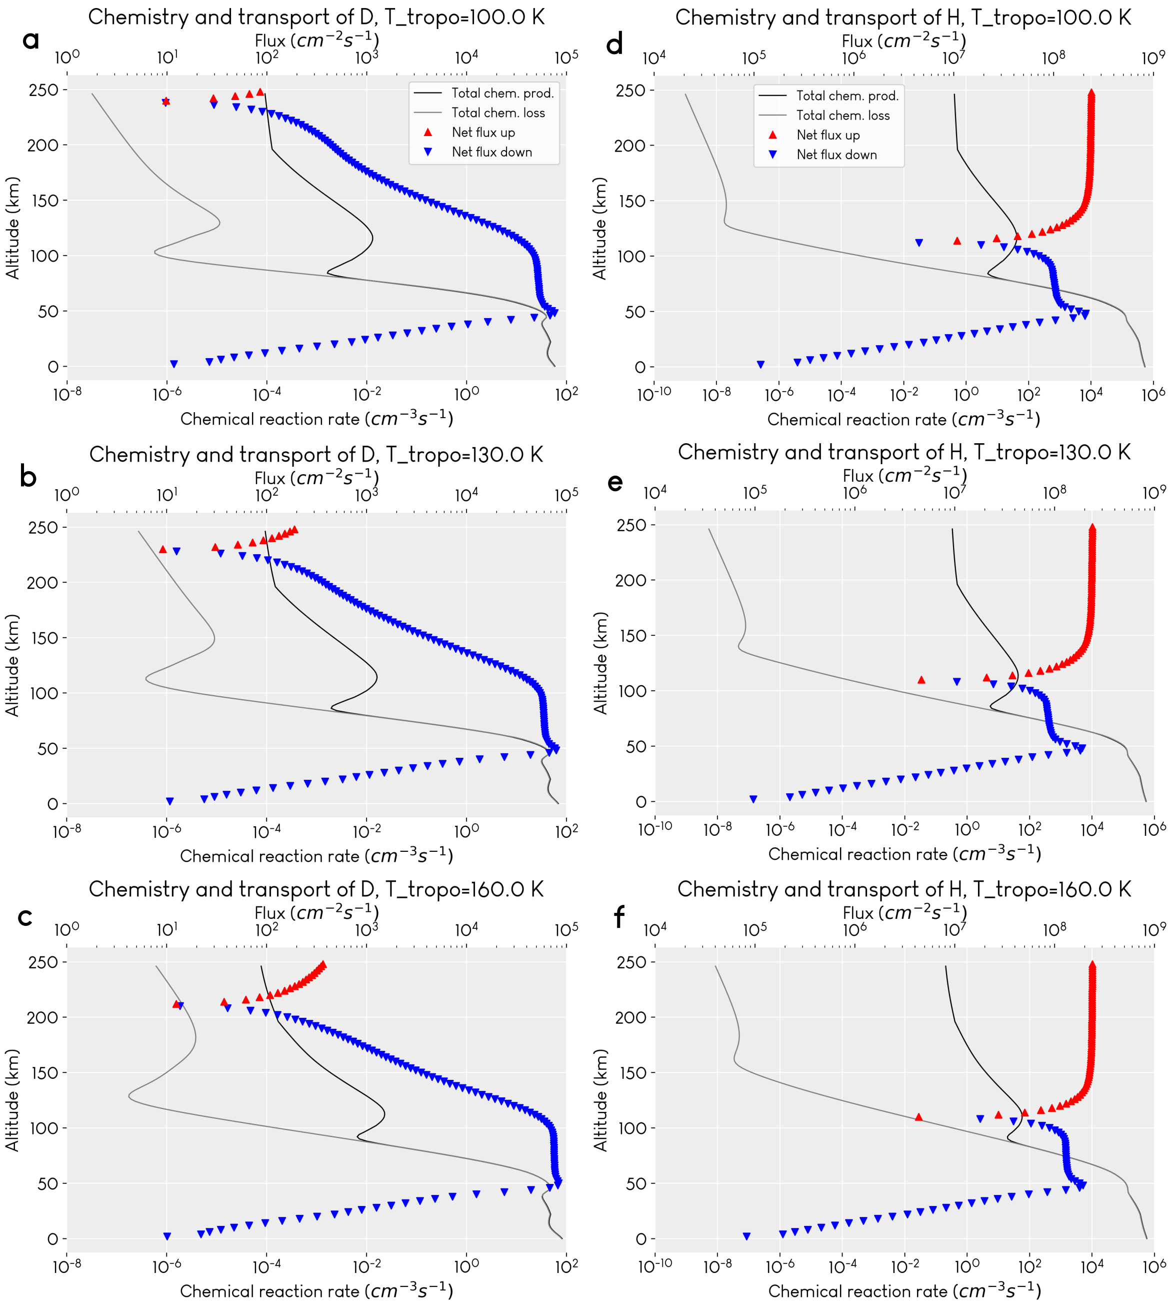


**Figure S6.** Chemical production and loss (bottom axis) and net flux (top axis) of atomic D (panels a, b, and c) and H (panels d, e, and f) as a function of the tropopause temperature $T_{\text{tropo}}$. As $T_{\text{tropo}}$ increases and $T_{\text{exo}}$ remains fixed, the thermosphere also warms, enabling greater upward flux (red triangles) at lower altitudes. D, which is not diffusion limited, responds strongly with increased escape flux and very weakly with increased loss via photochemistry. Because H takes up the lion's share of the $\phi_D + \phi_H = 2\phi_O$ required balance, its response is a relatively weak decrease (not visible in plot), to "make room" for the increased $\phi_D$.

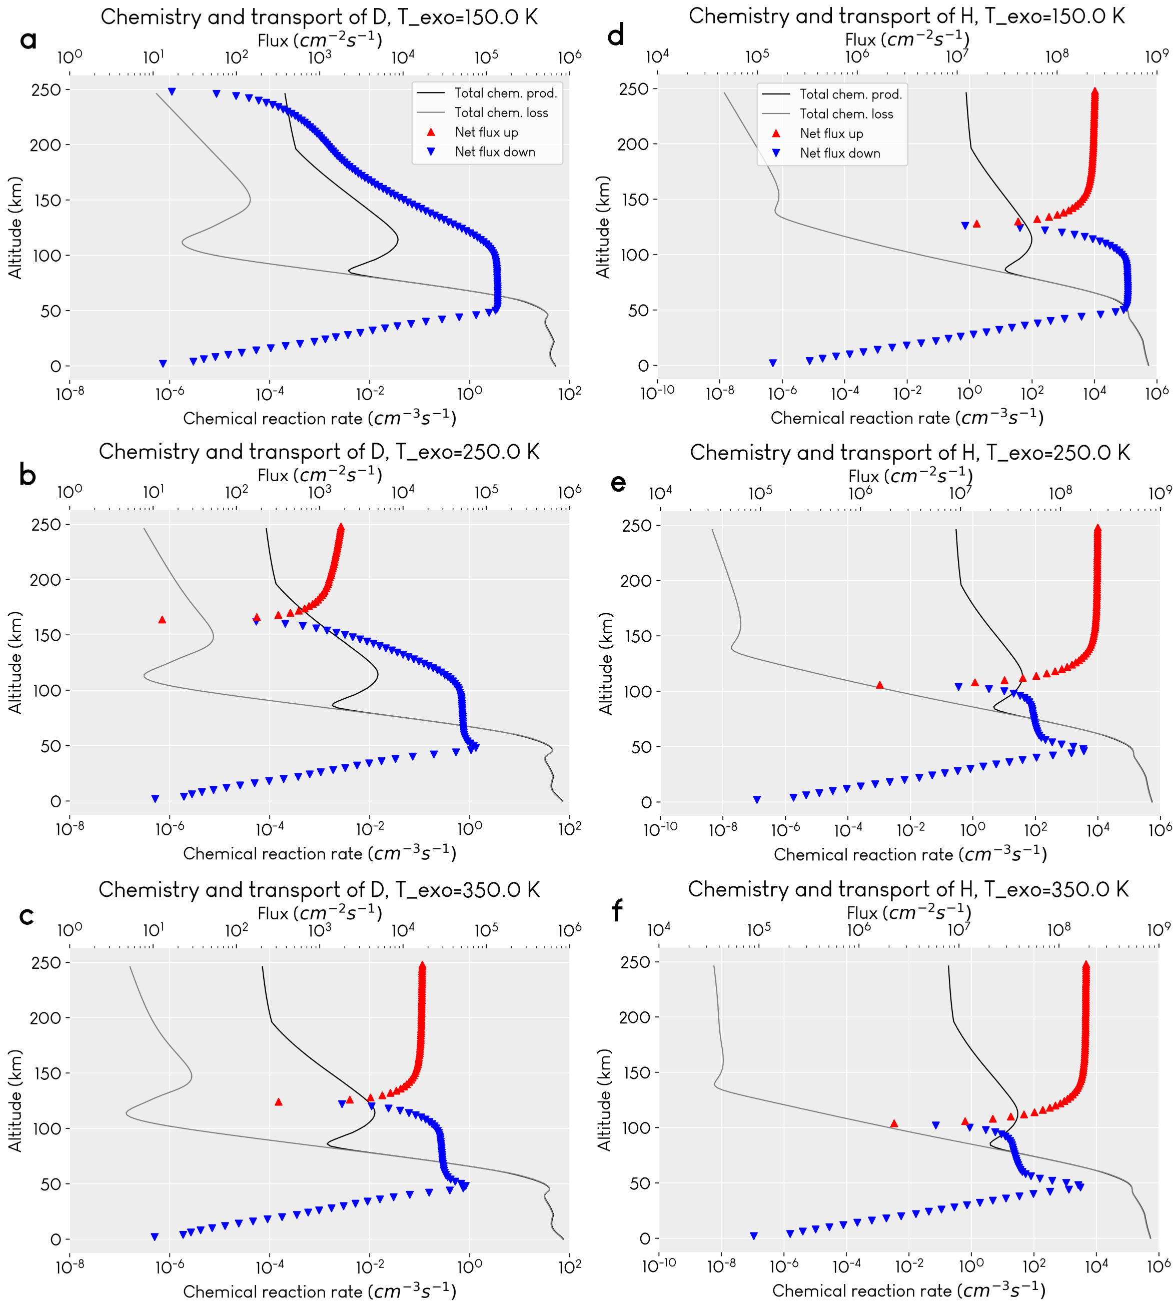


**Figure S7.** The same as Figure S5, but for $T_{\text{exo}}$. Here, the same mechanisms are more prominently shown, and the decrease in $\phi_H$ to "make room" for the increased $\phi_D$ according to the stoichiometric balance is just visible.
